# Supplementary material for: A Deep Moving-camera Background Model
Source: arXiv:2209.07923 source file (2022-09-16)
Supplement: Supplementary file 3 [file cpab.tex]

\section{Diffeomorphisms}

Following recent incorporations of diffeomorphisms in STNs~\cite{Skafte:CVPR:2018:DDTN,Balakrishnan:CVPR:2018:unsupervised,Dalca:NIPS:2019:learning},
 we also evaluate the benefits of applying diffeomorphic-STN for MCBM. 
 
 \begin{definition}
  A ($C^1$) diffeomorphism is a differentiable invertible map with a differentiable inverse. 
 \end{definition}

 The advantages these qualities (a differentiable invertible map with a differentiable inverse) had been shown to increase expressiveness
 in the produced warps while maintaining stability during the training phase of DL models~\cite{Skafte:CVPR:2018:DDTN}.
In practice, however, incorporating diffeomorphisms usually involves expensive computations which might hinder their use in DL-frameworks.
The reason is that during training, evaluations
of $x\mapsto T^\btheta(x)$ (forward pass) and $x\mapsto \nabla_\btheta T^\btheta( x)$ (backward pass)
are computed at multiple points $x$ and for multiple $\btheta$'s. 
To mitigate this effect, while still maintaining expressiveness, we decide to follow~\cite{Skafte:CVPR:2018:DDTN} and incorporate 
CPAB warps, which were recently proposed in~\cite{Freifeld:ICCV:2015:CPAB,Freifeld:PAMI:2017:CPAB}. 
These warps had shown to combine expressiveness and efficiency in DL context~\cite{Hauberg:AISTATS:2016:DA,Skafte:CVPR:2018:DDTN}. 
Additionally, diffeomorphic temporal transformer networks were shown to be effective in the joint-alignment 
of time-series data~\cite{Kaufman:ICIP:2021:cyclic,Lohit:CVPR:2019:temporal,Shapira:NIPS:2019:DTAN}.
Thus, we also utilize the diffeomorphic STN for the task of jointly-aligning frames when building the panorama for our MCBM.
Below we briefly explain CPAB warps and refer the reader to~\cite{Freifeld:ICCV:2015:CPAB,Freifeld:PAMI:2017:CPAB,Freifeld:TR_CPAB_Derivaitive:2017}
for more details. 

\RED{Ron: did not change the part below}

\textbf{CPAB transformations:} transformations which are Based on Piecewise-Affine (CPA-Based) velocity fields.
The term ``piecewise'' is \wrt some partition, denoted by $\Omega$, of the input's domain into sub-intervals.
Let $\Vcal$ denote the linear space of CPA velocity fields \wrt such a fixed $\Omega$,
let $d=\dim(\Vcal)$, and let $v^\btheta:\Omega\to\RR$, a velocity field parametrized
by $\btheta\in\Rd$, denote the generic element
of $\Vcal$, where $\btheta$ stands for the coefficient \wrt some basis of $\Vcal$.
The corresponding space of CPAB warps, obtained via integration of elements of $\Vcal$,  is 
\begin{align}
 \Tcal\triangleq&
 %\set
 \{T^\btheta:
   x\mapsto \phi^\btheta( x;1)
  \text{ s.t. } \phi^\btheta( x;t) \text{ solves }  \\
  %\phi^\btheta(x;t)
  =& x+\int_{0}^t  v^\btheta(\phi^\btheta(x;\tau))\, 
 \mathrm{d}\tau \text{ where }  v^\btheta\in \Vcal\, \};
 \label{Eqn:IntegralEquation}
\end{align}
it can be shown that these warps are indeed ($C^1$) diffeomorphisms~\cite{Freifeld:ICCV:2015:CPAB,Freifeld:PAMI:2017:CPAB}.
While $v^\btheta$
is CPA, $T^\btheta:\Omega\to\Omega$ is not (\eg, $T^\btheta$ is differentiable).
% Also note that $T^\btheta$ is not piecewise-quadratic: $v^\btheta$ is
% integrated as a velocity field, not as a function.
CPA velocity fields support an
integration method that is faster \emph{and} more accurate than typical 
velocity-field integration methods~\cite{Freifeld:ICCV:2015:CPAB,Freifeld:PAMI:2017:CPAB}.
The fineness of  $\Omega$ controls the trade-off between expressiveness of $\Tcal$
on the one hand and the associated computational complexity and dimensionality on the other 
hand. 
%
%
%

% \textbf{Initialization.} Since $\btheta = \bzero$ gives the identity map 
% we initialize the CPAB layer by setting all the weights in the 
% final layer of the localization net to zero.

% \textbf{Optional zero-boundary conditions}. If of interest, one can easily restrict 
% the CPA fields to vanish at the endpoints of the domain, implying these points will be fixed points
% of of the resulting warp. 
% Importantly in the TTN context, the \emph{CPAB gradient},
% $\nabla_\btheta T^\btheta( x)$, is given by the efficient solution of
% a system of coupled integral 
% equations~\cite{Freifeld:PAMI:2017:CPAB}; see~\cite{Freifeld:TR_CPAB_Derivaitive:2017}
%  for details.
