# Supplementary material for: A Deep Moving-camera Background Model
Source: arXiv:2209.07923 source file (2022-09-16)
Supplement: Supplementary file 5 [file prelims.tex]

\section{Spatial Transformer Networks} 
The Spatial Transformer Network (STN) \cite{Jaderberg:NIPS:2015:spatial} is a differentiable module that applies
 a parametrized spatial transformation in an input--dependent manner. 
Given a family of spatial transformations (\ie Affine) parametrized by $\btheta$ and an input image $U$, 
the STN predicts $\btheta$ and warps its input to produce $\mathcal{T}^{\btheta}(U)=V$ that minimize the loss of the downstream task.
The basic building blocks of the STN are as follows:
\begin{enumerate}
 \item \textbf{Localization network:} the localization network, $f_{\mathrm{loc}}$, is function which maps an input feature map $U$ to transformation 
 parameters $\btheta$, such that $f_{\mathrm{loc}}(\textbf{\textit{U}})=\btheta$. In the context of DL, $f_{\mathrm{loc}}$ is usually a regression
 neural network tasked to predict $\btheta$ by setting it's final layer to be $d=\dim(\btheta)$.
 \item \textbf{Parameterised Sampling Grid:} a sampling grid $G \subset[-1,1] \times$ $[-1,1]$ of evenly-spaced points corresponding 
 to the width and height ($xy$) of the input. $G$ is transformed by the transformation $T^{\btheta}$ and is later used to interpolate pixel-values from the input $U$.

 \item \textbf{Differentiable Image Sampling}. given $U, \btheta, \mathcal{T}$ and $G$, the sampler produce the output feature map $V$.
 A sampling kernel is applied to $U$ at $T^{\btheta}(G)$ to get the corresponding pixel value for the output $V$. 
 In practice, the inverse transformation is applied, $(T^{\btheta})^{-1}$, as specified in~\cite{Jaderberg:NIPS:2015:spatial}. 
 A popular choice is a bilinear sampling kernel.

\end{enumerate}
